# Supplementary material for: Clustering-based Partitioning for Large Web Graphs
Source: arXiv:2201.00472 source file (2022-01-03)
Supplement: Supplementary file 1 [file appendix.tex]

\section{Appendix}
%\newpage
%\appendix
\label{sec:app}
%\small
%\subsection{Proof}

\subsection{Submodularity and Non-decreasingness of Function $p^{(j)}$}
\label{sec:sub_non}
We show Lemmas~\ref{lem:psub} and \ref{lem:pinc}, which are on the properties of finishing probability functions.
Assume a set $S$ of executed subtasks, and a to-be-executed subtask $e$, satisfying $S \cap \left\{e\right\} = \emptyset$.
We define $p^S(\tau^{(j)})$ as the finishing probability of subtask $\tau^{(j)}$ given that the subtasks in $S$ are executed.

Similarly, we define $\rho_{err}^S(\tau^{(j)})$ and $I^S(\tau^{(j)})$ as the error ratio and the interpolation distance (i.e., $I^S(\tau^{(j)}) =\sum_{e \in S_{KNN}} |\tau^{(j)}, e|_i$) of subtask $\tau^{(j)}$, respectively, given that all subtasks in $S$ are executed.
%j$I^S(\tau^{(j)})$ as the interpolation distance of subtask $\tau^{(j)}$ with the executed subsets $S$.
Without causing any ambiguities, in the proofs, we simplify $\rho_{err}^S(\tau^{(j)})$ and $I^S(\tau^{(j)})$ as $\rho_{err}^S$ and $I^S$, respectively.
%(We simplify $\rho_{err}^S(\tau^{(j)})$ to $\rho_{err}^S$, and $I^S(\tau^{(j)})$ to $I^S$.)

\begin{lemma}
\label{lem:psub}
The function $p^{(j)}$ is submodular.
\end{lemma}

\begin{proof}
%jWe prove the finishing probability function $p^{(j)}$ is submodular by proving the error rate function $\rho_{err}(\tau^{(j)})$ is submodular. The finishing probability function $p^{(j)}$ is submodular if:
To prove function $p^{(j)}$ is submodular, it is equivalently to prove the following.
\begin{equation}
\label{proof:pj}
p^{ S \cap \left\{ e \right\} } (\tau^{(j)}) +  p^{S \cup \left\{ e \right\}} (\tau^{(j)}) \leq p^S (\tau^{(j)}) + p^{ \left\{ e \right\} } (\tau^{(j)})
\end{equation}
By substituting it with Equation~\ref{eqn:p}, we can rewrite it as $\rho_{err}^{ S \cap \left\{ e \right\} }  +  \rho_{err}^{S \cup \left\{ e \right\}}  \geq \rho_{err}^S  + \rho_{err}^{ \left\{ e \right\} }
$.% follows.
%\begin{equation}
%\rho_{err}^{ S \cap \left\{ e \right\} }  +  \rho_{err}^{S \cup \left\{ e \right\}}  \geq \rho_{err}^S  + \rho_{err}^{ \left\{ e \right\} }
%\end{equation}
Equivalently, it is sufficient to prove that
%$\rho_{err}^{ S \cap \left\{ e \right\} }  +  \rho_{err}^{S \cup \left\{ e \right\}} - \rho_{err}^S  - \rho_{err}^{ \left\{ e \right\} } \geq 0$.
\begin{equation}
\label{pf:rho}
\rho_{err}^{ S \cap \left\{ e \right\} }  +  \rho_{err}^{S \cup \left\{ e \right\}} - \rho_{err}^S  - \rho_{err}^{ \left\{ e \right\} } \geq 0
\end{equation}
From Equation~\ref{eqn:rho}, we know that $\rho_{err}$'s value is dependent on the $\tau^{(j)}$'s $k$-NN set, $S_{KNN}$, which must be a subset of $S$.
Next, we show the correctness of Equation~\ref{pf:rho}, by enumerating all three possible case of $S$.
%The set $S$ has three situations, respectively, $S = \emptyset$, $0<|S|<k$, $S \geq k$, and we prove equation \ref{pf:rho} from these three aspects.

{\it Case} 1.  When $S = \emptyset$, we have
%$\rho_{err}^{ S \cap \left\{ e \right\} } = \rho_{err}^S $, $ \rho_{err}^{S \cup \left\{ e \right\}} = \rho_{err}^{ \left\{ e \right\} }$,
$\rho_{err}^{ S \cap \left\{ e \right\} }  +  \rho_{err}^{S \cup \left\{ e \right\}} - \rho_{err}^S  - \rho_{err}^{ \left\{ e \right\} } = 0$, and thus Equation \ref{pf:rho} holds.

{\it Case} 2.  When $0<|S|<k$,  we have
$\rho_{err}^{ S \cap \left\{ e \right\} } = 1$ and $\rho_{err}^{ \left\{ e \right\} } = 1 - \frac{1}{k} + \frac{I^{ \left\{ e \right\} }}{km}$.
Here, $\rho_{err}^{S \cup \left\{ e \right\}}$ has two subcases, depending on $|S|$.

The subcase (a) refers to $|S|=k-1$. In that case, there are $k$ finished subtasks after executing $e$. Then, $ \rho_{err}^{S \cup \left\{ e \right\}} = \frac{I^{S \cup \left\{ e \right\}}}{km}$, and $\rho_{err}^S = \frac{I^S}{km} +  \frac{1}{k}$. We can have $\rho_{err}^{ S \cap \left\{ e \right\} }  +  \rho_{err}^{S \cup \left\{ e \right\}} - \rho_{err}^S  - \rho_{err}^{ \left\{ e \right\} } =  \frac{I^{S \cup \left\{ e \right\}}}{km} - \frac{I^S}{km} - \frac{I^{\left\{ e \right\}}}{km} = 0$.
%As $I^{S \cup \left\{ e \right\}} = I^S + I^{\left\{ e \right\}}$, the equation \ref{pf:rho} $ = 0$.
Equation~\ref{pf:rho} holds.

The subcase (b) means that the total number of finished subtasks does not exceed $k$, after executing subtask $e$. Thus, we have $ \rho_{err}^{S \cup \left\{ e \right\}} = 1 - \frac{|S|+1}{k} + \frac{I^{S \cup \left\{ e \right\}}}{km}$ and $\rho_{err}^S = 1 - \frac{|S|}{k} + \frac{I^S}{km}$.
Then, $\rho_{err}^{ S \cap \left\{ e \right\} }  +  \rho_{err}^{S \cup \left\{ e \right\}} - \rho_{err}^S  - \rho_{err}^{ \left\{ e \right\} } = \frac{I^{S \cup \left\{ e \right\}}}{km}  - \frac{I^S }{km} - \frac{I^{\left\{ e \right\}}}{km}  = 0$. Equation \ref{pf:rho} holds.

{\it Case} 3. When $|S| \geq k$,  $\rho_{err}^{ S \cap \left\{ e \right\} } = 1$, we have $\rho_{err}^{ \left\{ e \right\} } = 1 - \frac{1}{k} + \frac{I^{ \left\{ e \right\} }}{km}$, $\rho_{err}^S = \frac{I^S}{km}$, and $ \rho_{err}^{S \cup \left\{ e \right\}} = \frac{I^{S \cup \left\{ e \right\}}}{km} $.
Based on whether the execution of subtask $e$ changes $S_{KNN}$ ($\tau^{(j)}$'s $k$-NN set), there can be two subcases.

If $S_{KNN}$ is not affected by $e$, we have that $ \rho_{err}^{S \cup \left\{ e \right\}} =\rho_{err}^S$. So, $\rho_{err}^{ S \cap \left\{ e \right\} }  +  \rho_{err}^{S \cup \left\{ e \right\}} - \rho_{err}^S  - \rho_{err}^{ \left\{ e \right\} } = \rho_{err}^{ S \cap \left\{ e \right\} } - \rho_{err}^{ \left\{ e \right\} } =  \frac{1}{k} - \frac{I^{ \left\{ e \right\} }}{km}$.
As the interpolation distance $I^{ \left\{ e \right\} }$ is less than $m $, we have $\frac{1}{k} - \frac{I^{ \left\{ e \right\} }}{km} >0$.
So, Equation \ref{pf:rho} holds.

If $S_{KNN}$ is affected by $e$, it implies that a subtask in $S_{KNN}$ is updated by $e$. Suppose the replaced subtask in original $S_{KNN}$ be $e'$, and the updated interpolation distance be $ I^{S \cup \left\{ e \right\}} = I^S - I^{\left\{ e' \right\}} + I^{ \left\{ e \right\} }$.
We can have $\rho_{err}^{ S \cap \left\{ e \right\} }  +  \rho_{err}^{S \cup \left\{ e \right\}} - \rho_{err}^S  - \rho_{err}^{ \left\{ e \right\} } = \frac{I^{S \cup \left\{ e \right\}}}{km} - \frac{I^S}{km} + \frac{1}{k} - \frac{I^{ \left\{ e \right\} }}{km} =  \frac{1}{k} - \frac{I^{ \left\{ e' \right\} }}{km} $. As the interpolation distance $I^{ \left\{ e' \right\} }$ is less than $m$, we have $\frac{1}{k} - \frac{I^{ \left\{ e' \right\} }}{km} >0$. Equation \ref{pf:rho} holds.

In summary, Equation \ref{pf:rho} holds in all three cases. The lemma is proved.
\end{proof}

\begin{lemma}
\label{lem:pinc}
The function $p^{(j)}$ is non-decreasing.
\end{lemma}

\begin{proof}
We prove the finishing probability function $p^{(j)}$ is non-decreasing by showing that the error rate function $\rho_{err}(\tau^{(j)})$ is non-increasing. Or, equivalently, %$\rho_{err}^{S \cup \left\{ e \right\}} - \rho_{err}^S \leq 0$.
%The error rate function $\rho_{err}(\tau^{(j)})$ is non-increasing if
\begin{equation}
\label{pf:non_increase}
\rho_{err}^{S \cup \left\{ e \right\}} - \rho_{err}^S \leq 0
\end{equation}
There can be two possible cases for set $S$, $0 \leq |S|<k$ and $|S| \geq k$. We hereby prove the correctness of Equation~\ref{pf:non_increase} by considering the two cases.

{\it Case} 1. When $0 \leq |S|<k$,  $ \rho_{err}^{S \cup \left\{ e \right\}}$ have two subcases, depending on the size of set $S$.

The first subcase is for $|S|=k-1$, and thus the total subtasks number is $k$ after adding the executed subtask $e$. Then, $ \rho_{err}^{S \cup \left\{ e \right\}} = \frac{I^{S \cup \left\{ e \right\}}}{km}$, and $\rho_{err}^S = \frac{I^S}{km} +  \frac{1}{k}$. So, we have $\rho_{err}^{S \cup \left\{ e \right\}} - \rho_{err}^S = \frac{ I^{S \cup \left\{ e \right\}}}{km} - \frac{I^S}{km} - \frac{1}{k} = \frac{I^{\left\{ e \right\}}}{km} - \frac{1}{k}$. As the interpolation distance $I^{ \left\{ e \right\} }$ is less than $m $,  Equation \ref{pf:non_increase} holds.

The second subcase is for $|S| < k-1$, meaning that the total number of subtasks is less than $k$ after the execution of $e$.
We can thus have $ \rho_{err}^{S \cup \left\{ e \right\}} = 1 - \frac{|S|+1}{k} + \frac{I^{S \cup \left\{ e \right\}}}{km}$, and  $\rho_{err}^S = 1 - \frac{|S|}{k} + \frac{I^S}{km}$. So, $ \rho_{err}^{S \cup \left\{ e \right\}} - \rho_{err}^S  = \frac{I^{S \cup \left\{ e \right\}}}{km}  - \frac{I^S}{km}  - \frac{1}{k} = \frac{I^{\left\{ e \right\}}}{km} - \frac{1}{k}$. Equation \ref{pf:non_increase} holds.

{\it Case} 2. When $S \geq k$, we can have $\rho_{err}^S = \frac{I^S}{km}$ and $ \rho_{err}^{S \cup \left\{ e \right\}} = \frac{I^{S \cup \left\{ e \right\}}}{km} $.
Based on whether the execution of subtask $e$ changes $S_{KNN}$, there can be two subcases.

If $S_{KNN}$ is not affected by $e$, we have $ \rho_{err}^{S \cup \left\{ e \right\}} =\rho_{err}^S$, so that Equation \ref{pf:non_increase} holds.

If $S_{KNN}$ is affected by $e$, it means that a subtask in $S_{KNN}$ is updated by $e$. We denote the replaced subtask in original $S_{KNN}$ as $e'$, and the updated interpolation distance as $ I^{S \cup \left\{ e \right\}} = I^S - I^{\left\{ e' \right\}} + I^{ \left\{ e \right\} }$.
%We get that $ I^{S \cup \left\{ e \right\}} = I^{S - \left\{ e' \right\}} + I^{ \left\{ e \right\} }$ and $I^S = I^{S - \left\{ e' \right\}} + I^{ \left\{ e' \right\} }$.
Then, we can get $\rho_{err}^{S \cup \left\{ e \right\}} - \rho_{err}^S  = \frac{I^{S \cup \left\{ e \right\}}}{km} - \frac{I^S}{km}  =  \frac{I^{ \left\{ e \right\} }}{km} - \frac{I^{ \left\{ e' \right\} }}{km} $.
More, the fact that $e'$ is replaced by $e$ implies that $I^{ \left\{ e \right\} } < I^{ \left\{ e' \right\} }$. So, Equation \ref{pf:non_increase} holds.

In summary, Equation \ref{pf:non_increase} holds in all possible cases. Hence, the lemma is proved.
\end{proof}

\subsection{Proof of Lemma~\ref{lem:cond1}}
\label{subsec:cond1}

\begin{lemma}
\label{lem:cond1}
For a time segment $[l, r]$, if $knn(l)=knn(r)$, it is true that $\forall e \in [l, r], knn(e) = knn(l) = knn(r)$.
\end{lemma}

\begin{proof}
We prove that by contradiction. Assume a time segment $[l,r]$, $NN(l) = NN(r)$, and a slot $e$ on the segment, $e \in [l,r]$, $NN(l) \neq NN(e)$. We use $a$ and $b$ denote $NN(l)$ and $NN(e)$, $a \neq b$, $|b,e|_t <|a, e|_t$, and $b$ is in the range of $(e-|a,e|_t, e+|a,e|_t)$(It doesn't include two endpoints). According to the position of $a$, it can be divided into three cases:

The first case is for $l \leq a \leq r$. As $a$ is the $NN$ of $l$ and $r$, there is no other executed subtask within the time segment $[l-|l,a|_t, r+|r,a|_t]$. It has $e-|a,e|_t - (l-|l,a|_t) = |l,e|_t  -|a,e|_t + |l,a|_t \geq 0 $ and $r+|r,a|_t - (e+|a,e|_t) = |r,e|_t - |a,e|_t + |r, a|_t \geq 0 $, then the range of $b$ is within the range $[l-|l,a|_t, r+|r,a|_t]$. The case can not exist.

The second case is for $a < l$, and the range of $b$ is $(e, e+|a,e|_t)$. As $a$ is the $NN$ of $l$ and $r$, there is no other executed subtask within the time segment $(a, r + |a,r|_t)$, then the range of $b$ is within the range $(a, r + |a,r|_t)$. The case can not exist.

The third case is for $a > r$, then the range of $b$ is $(e-|a,e|_t, a)$. As $a$ is the $1-nn$ of $l$ and $r$, there is no other executed subtask within the time segment $(l - |a,l|_t, a)$, then the range of $b$ is within the range $(l - |a,l|_t, a)$. The case can not exist.
\end{proof}
